# Supplementary material for: Amodal Panoptic Segmentation
Source: arXiv:2202.11542 source file (2022-02-23)
Supplement: Supplementary file 1 [file appendix.tex]

%%%%%%%%%% Merge with supplemental materials %%%%%%%%%%
\clearpage

\setlength{\belowcaptionskip}{0pt}

\begin{center}
\vspace{-5ex}
\textbf{\LARGE \bf
Amodal Panoptic Segmentation} \\
\vspace{2ex}

\Large{\bf- Supplementary Material -}\\
\vspace{0.4cm}
\rohit {Fix title, add abstract}
\end{center}
\setcounter{section}{0}
\setcounter{equation}{0}
\setcounter{figure}{0}
\setcounter{table}{0}
\setcounter{page}{1}
\makeatletter

\section{Dataset Statistics}

\section{Baselines}

\section{Training Losses}

\section{Metric Analysis}
